# Supplementary material for: Rule-based OWL Modeling with ROWLTab Protege Plugin
Source: arXiv:1808.10108 source file (2018-08-30)
Supplement: Supplementary file 1 [file appendix.tex]

\section{Proofs}\label{section:davidApp}

Missing proofs etc.

%%% Local Variables:
%%% mode: latex
%%% TeX-master: "main"
%%% End:
